# Supplementary material for: Differentially Describing Groups of Graphs
Source: arXiv:2201.04064 source file (2022-03-10)
Supplement: Supplementary file 1 [file appendix.tex]

% !TeX spellcheck = en_US
% !TeX root = ../paper_appendix.tex
\section{Appendix} \label{sec:apx}

In this Appendix, we give an overview of our notation, 
derive our heuristic, 
and provide additional information on our experiments using synthetic and real-world data.

\subsection{Notation}

\begin{table}[h!]
	\centering
	\caption{%
		Overview of our notation.
	}\label{tab:notation}
	% !TeX spellcheck = en_US
% !TeX root = ../paper_appendix.tex
\begin{tabular}{rl}\toprule
	\bfseries Symbol&\bfseries Definition \\\midrule
	$\cG$ & Set of graphs\\
%	\color{red} $j$ ($N$) $\rightarrow$ $|\cG|$& $|\cG|$\\
	$\Pi$ & Partition of $\cG$\\
	$k$& $|\Pi|$\\ % was l intermittently
	$\cG_i$ & Group of graphs, $\cG_i\subseteq \cG$, $\cG_i\in \Pi$\\
	$c_i$&$|\cG_i|$\\
	$G_i$ & $(V,E_i)$, graph $i$\\
	$V$ & Node set (the same across all graphs)\\
	$n$  & $|V|$\\
	$E_i$& Edge set of graph $i$\\
	$m_i$&$|E_i|$\\
	$W$&Edge categories or discrete edge weights\\
	$\cE$&$V \times V \times W$\\
	$2^{\cE}$&Power set of $\cE$\\
	$X$ &Set of edges, $X\subseteq \cE$\\
	$V_X$&Set of nodes incident with an edge in $X$\\
	$q_i(X)$&Empirical frequency of $X$ in $\cG_i$\\
	$S$&Set of edge sets, $S\subseteq 2^{\cE}$\\
	$p_i(X\mid S)$&Expected frequency of $X$ in $\cG_i$ under $S$\\
	$f$&Maximum entropy distribution\\
	$\theta_i$&Real-valued model parameter\\
	$A$&Association matrix\\
	$S_i$&$\{X\in S \mid A_{iX} = 1\}$\\
	$\ell(S)$&Log likelihood of $S$\\
	$\Delta(X)$&$\ell(S) - \ell(S \cup \{X\}) - |\Pi|/2\log |\cG| $\\
	$h(X)$&Heuristic approximation of $\Delta(X)$\\
	$\gamma$&Largest connected component size of $G\in \cG$\\
	\bottomrule
\end{tabular}
\end{table}

\subsection{Heuristic}

% $$
% (k \cdot (|S \cup \{X\}|))/2 \log |\cG|  - (k \cdot |S|)/2 \log |\cG|  
% = 
% (k \cdot (|S| + 1))/2 \log |\cG|  - (k \cdot |S|)/2 \log |\cG|  
% =
% k/2 \log |\cG|
% $$

Starting with $\Delta(X)$, 
and abbreviating the constant model cost delta $k/2 \cdot |S \cup \{X\}| \cdot \log |\cG| - k/2 \cdot |S| \cdot \log |\cG|  
= k/2 \log |\cG|$ as $c$, we obtain
\begin{align*}
    \Delta(X) &= \ell(S) - \ell(S \cup \{X\}) - c \\
                &= -\sum_i \sum_{G \in \cG_i} \log p_i(G \mid S) - \log p_i(G \mid S \cup \{X\}) - c\\
                &= -\sum_i \sum_{G \in \cG_i} \log \frac{p_i(G \mid S)}{p_i(G \mid S \cup \{X\})} - c\;.\\
\end{align*}
Now, by constraining the sum to include only graphs in which $X$ is fully present, we get
{\small\begin{align*}
	-\sum_i \sum_{G \in \cG_i, X \subseteq G} \log \frac{p_i(X \mid S)}{p_i(X \mid S \cup \{X\})}\frac{p_i(G \setminus \{X\} \mid S)}{p_i(G \setminus \{X\} \mid S \cup \{X\})} - c\;,
\end{align*}}

\noindent using a factorization of $p$ and $G$.
By assuming that $\log \frac{p_i(G \setminus \{X\} \mid S)}{p_i(G \setminus \{X\} \mid S \cup \{X\})} \approx 0$, 
and since $p_i(X \mid S \cup \{X\}) = q_i(X)$ holds, 
we can further simplify the above to
\begin{align*}
	&-\sum_i c_i \cdot q_i(X) \log \frac{p_i(X \mid S)}{q_i(X)} - c\\
	&=\sum_i c_i \cdot q_i(X) \log \frac{q_i(X)}{p_i(X \mid S)} - c\quad \equiv h(X)\;,
\end{align*}
thus arriving at our heuristic.

\subsection{Experiments}

\subsubsection{Synthetic Data}

\begin{table}[b!]
	\caption{%
		Synthetic graph group configurations. 
		$k$ is the number of groups, $p$ is the edge probability in a $G(n,p)$ random graph model, $P$ is the pattern (\emph{cl}ique, \emph{st}ar, or \emph{b}i\emph{c}lique), and $|P|$ is the size of (the node equivalence classes in) the pattern. 
		\emph{Prevalence} is the occurrence probability of the pattern in the graph group, 
		\emph{position} is the label of the first node in the pattern,
		and \emph{t} indicates the pattern \emph{t}ype, 
		i.e., whether it is \emph{s}hared, \emph{o}verlapping, or \emph{c}ontrastive between graph groups.}\label{tab:synthetic}
	\centering
	% !TeX spellcheck = en_US
% !TeX root = paper_appendix.tex
	\begin{tabular}{rrcccc}
	\toprule
	\bfseries $k$& $p$ &\bfseries $P(|P|)$ & \bfseries Prevalence & \bfseries Position & $t$\\
	\midrule
	\multirow{2}{*}{$1$}&$0.2$&\multirow{2}{*}{\tiny\setlength\arraycolsep{1.5pt}$\begin{bmatrix}
		\text{cl}(5)\\\text{st}(1,9)\\\text{bc}(5,5)
	\end{bmatrix}$}&\setlength\arraycolsep{1.5pt}\tiny$\begin{bmatrix}
0.2&0.2&0.2
\end{bmatrix}^T$&\multirow{2}{*}{\setlength\arraycolsep{1.5pt}\tiny$\begin{bmatrix}
	0\\5\\15
\end{bmatrix}$}&\multirow{2}{*}{--}\\
	&$0.1$&&\setlength\arraycolsep{1.5pt}\tiny$\begin{bmatrix}
		0.1&0.2&0.3
	\end{bmatrix}^T$&&\\
	\midrule
	\multirow{3}{*}{$2$}&\multirow{3}{*}{$0.2$}&\multirow{3}{*}{$\text{st}(1,9)$}&\setlength\arraycolsep{1.5pt}$\begin{bmatrix}
		0.2&0.2
	\end{bmatrix}$&\setlength\arraycolsep{1.5pt}$\begin{bmatrix}
	0&0
\end{bmatrix}$&s\\
	&&&\setlength\arraycolsep{1.5pt}$\begin{bmatrix}
		0.2&0.4
	\end{bmatrix}$&\setlength\arraycolsep{1.5pt}$\begin{bmatrix}
	0&0
\end{bmatrix}$&c\\
	&&&\setlength\arraycolsep{1.5pt}$\begin{bmatrix}
		0.4&0.4
	\end{bmatrix}$&\setlength\arraycolsep{1.5pt}$\begin{bmatrix}
	0&10
\end{bmatrix}$&c\\
	\midrule
	\multirow{3}{*}{$2$}&\multirow{3}{*}{$0.2$}&\multirow{3}{*}{$\text{cl}(5)$}&\multirow{3}{*}{\setlength\arraycolsep{1.5pt}$\begin{bmatrix}
		0.2&0.2
	\end{bmatrix}$}&\setlength\arraycolsep{1.5pt}$\begin{bmatrix}
0&0
\end{bmatrix}$&s\\
 	&&&&\setlength\arraycolsep{1.5pt}$\begin{bmatrix}
 		0&2
 	\end{bmatrix}$&o\\
	&&&&\setlength\arraycolsep{1.5pt}$\begin{bmatrix}
		0&5
	\end{bmatrix}$&c\\
	\midrule
	\multirow{5}{*}{$4$}&$0.2$&\multirow{5}{*}{\tiny\setlength\arraycolsep{1.5pt}$\begin{bmatrix}
		\text{cl}(5)\\\text{cl}(5)\\\text{st}(1,9)\\\text{st}(1,9)\\\text{bc}(5,5)
	\end{bmatrix}$}&
	\tiny\setlength\arraycolsep{1.5pt}$\begin{bmatrix}
		0.2 & 0.2 & 0 & 0 & 0\\
		0 & 0.2 & 0.2 & 0 & 0\\
		0 & 0 & 0.2 & 0.2  & 0\\
		0 & 0 & 0 & 0.2 & 0.2\\
	\end{bmatrix}^T$&\multirow{5}{*}{\tiny\setlength\arraycolsep{1.5pt}$\begin{bmatrix}
	0\\5\\10\\20\\30
\end{bmatrix}*4$}&\multirow{5}{*}{\tiny\setlength\arraycolsep{1.5pt}$\begin{bmatrix}
\text{c}\\\text{s}\\\text{s}\\\text{s}\\\text{c}
\end{bmatrix}$}\\
&&&&&\\
	&$0.1$&&\tiny\setlength\arraycolsep{1.5pt}$\begin{bmatrix}
		0.1 & 0.2 & 0 & 0 & 0\\
		0 & 0.1 & 0.2 & 0 & 0\\
		0 & 0 & 0.3 & 0.2  & 0\\
		0 & 0 & 0 & 0.3 & 0.2\\
	\end{bmatrix}^T$&&\\
	\bottomrule
\end{tabular}
\end{table}

For each configuration from Tab.~\ref{tab:synthetic}, 
we generate $100$ graph group datasets with $k\in \{1,2,4\}$ graph groups.
Each group consists of $100$ graphs with $n = 100$ nodes (labeled from $0$ to $99$), 
and edges are sampled randomly using a $G(n,p)$ random graph model, 
edge probability $p\in\{0.1,0.2\}$, and different seeds. 
We then plant \emph{cliques} (i.e., complete graphs) of size $5$, 
\emph{stars} (i.e., one hub node connected to pairwise nonadjacent spoke nodes) of size $10$, 
and balanced \emph{bicliques} (i.e., two equally sized independent node sets $A$ and $B$ such that every node in $A$ is connected to every node in $B$) of size $10$
as patterns into these random graphs, 
using the prevalence and position parameters given in the fourth and fifth columns of Tab.~\ref{tab:synthetic}.
Here, each column in the prevalence and position matrices corresponds to a graph group, 
and repeated columns in the four-group setting are condensed as $[\cdot]*4$.

For example, for the second one-group setting (Tab.~\ref{tab:synthetic}, Row~$2$), 
we plant a clique starting at node $0$ with prevalence $0.1$, 
a star starting at node $5$ with prevalence $0.2$, 
and a biclique starting at node $15$ with prevalence $0.3$,
into $100$ graphs generated using $G(100,0.1)$.

As described in the main paper and mirrored in the layout of Tab.~\ref{tab:synthetic}, 
we distinguish three scenarios: 
the one-group, the two-group, and the four-group scenario.
In each scenario, we evaluate the performance of \ourmethod, $\ourmethod_{\text{BIC}}$, and---in the two-group setting---its competitors, 
using precision, recall, and F1 score for the edges of the planted patterns. 
We compute these statistics based on the edge sets of the planted patterns for each graph group dataset separately, 
and report the result distributions in Fig.~$2$ from the main paper.

\subsubsection{Real-world Data}

We use real-world data from three different domains: 
functional brain networks (fbn), 
air transportation networks (atn), 
and international trade networks (itn). 
Functional brain networks are modeled as undirected, unweighted graphs, 
whereas both air transportation networks and international trade networks 
are modeled as directed, weighted graphs, 
with ten discrete weight categories created using equal-width binning.

The functional brain network data stem from the Autism Brain Imaging Data Exchange (ABIDE).
In the graphs representing these data,
each node corresponds to a region of interest (ROI) from the automated anatomical labeling (AAL) atlas, 
and each unweighted, undirected edge corresponds to a relatively strong blood-oxygen-level dependent (BOLD) signal correlation between the time series of these regions obtained during a resting-state functional magnetic resonance imaging (fMRI) scanning session.
Here, our data consists of one graph per subject.
Subjects can be partitioned by their \emph{diagnostic status} (either ASD if diagnosed with autism spectrum disorder or TD if typically developed), 
and they can be grouped or selected by other attributes, 
such as \emph{sex} (the only options being male and female),
\emph{age}, or \emph{scanning modality} (eyes open or eyes closed).

The air transportation network data are taken from the website of the Bureau of Transportation Statistics (BTS).
In the graphs representing these data, 
each node corresponds to an airport in the United States, 
and each weighted, directed edge corresponds to the volume of a passenger flow.
Here, our data consists of one graph per \emph{carrier class} and \emph{month} from $2005$ to $2020$ ($374$ graphs in total). 

The international trade network data are sourced from the World Integrated Trade Solution (WITS) provided by the World Bank.
In the graphs representing these data, 
each node corresponds to a country (or similar unit), 
and each weighted, directed edge corresponds to the value of a trade flow.
Here, our data consists of one graph per \emph{product class} (Animals, Vegetables, Food Products, Minerals, or Chemicals) and \emph{month} from $1989$ to $2018$ ($3\,976$ graphs in total). 

We run \ourmethod on different subsets and splits of our datasets 
as shown in the three sections of Tab.~\ref{tab:data}.

\newpage

\begin{table}[h!]
	\caption{%
		Real-world graph group data used in our experiments. 
		$n$ is the number of nodes, $[m]$ specifies the range of the number of edges per graph, 
		$k$ is the number of graph groups, 
		and $[c_i]$ specifies the range of the group cardinalities. 
		\emph{TD} stands for \emph{Typically Developed}, 
		and \emph{ASD} stands for \emph{Autism Spectrum Disorder}.
		For the brain networks, which are sparsified during preprocessing, we use a minimum support of $2$, 
		and for the airline transportation networks and the international trade networks, 
		we use an adaptive threshold of $0.1$ times the cardinality of the smallest group in the experiment for sparsification. 
		In all experiments, we use Vuong's test at a conservative significance level of $1\times 10^{-7}$ (or $1 \times 10^{-5}$ when operating with less than $50$ samples).
	}\label{tab:data}
	\centering
	% !TeX spellcheck = en_US
% !TeX root = paper_appendix.tex
\begin{tabular}{p{0.13\linewidth}p{0.4125\linewidth}rr}
	\toprule
	\bfseries \mbox{Dataset}& \bfseries Description & $k$ & $[c_i]$\\
	\midrule
	\multicolumn{4}{c}{Functional Brain Networks (undirected, unweighted)}\\
	\multicolumn{4}{c}{$n = 116$; $m\in[1\,320,1\,348]$}\\
	\midrule
	fbn-a&\mbox{TD vs. ASD, age $[15,20]$}&$2$&$[116,121]$\\
	fbn-a1&\mbox{ASD, age $[15,20]$}&$1$&$[116]$\\
	fbn-c&TD vs. ASD, age $\leq 9$&$2$&$[49,52]$\\
	fbn-c1&ASD, age $\leq 9$&$1$&$[49]$\\
	fbn-ac&TD vs. ASD~$\times$~a vs. c&$4$&$[49,121]$\\
	fbn-e&\mbox{TD vs. ASD, eyes closed}&$2$&$[136,158]$\\
	fbn-e1&ASD, eyes closed&$1$&$[136]$\\
	fbn-m&TD vs. ASD, males only&$2$&$[418,420]$\\
	fbn-m1&ASD, males only&$1$&$[420]$\\
	\midrule
	\multicolumn{4}{c}{Air Transportation Networks (directed, weighted)}\\ 
	\multicolumn{4}{c}{$n = 300$; $m\in [335,3\,533]$}\\
	\midrule
	atn&all $(2005$--$2020)$&$1$&$[374]$\\
	atn-m&major carriers&$1$&$[191]$\\
	atn-n&national carriers&$1$&$[183]$\\
	atn-c&carrier classes&$2$&$[183,191]$\\
	%atn-s&season $[10,3]$ vs. $[4,9]$&$2$&$[185,189]$\\
	%atn-sc&season and carrier class&$4$&$[90,96]$\\
	%atn-q1&quarters from Jan&$4$&$[92,95]$\\
	atn-q&quarters $[12,3,6,9)$&$4$&$[92,95]$\\
	%atn-q3&quarters from Nov&$4$&$[93,94]$\\
	atn-y&four-year intervals&$4$&$[86,96]$\\
	\midrule
	\multicolumn{4}{c}{International Trade Networks (directed, weighted)}\\
	\multicolumn{4}{c}{$n = 250$; $m\in [256,11\,415]$}\\
	\midrule
	itn&all $(1989$--$2018)$&$1$&$[3\,976]$\\
	itn-p&product class&$5$&$[210,1\,530]$\\
	itn-y&ten-year intervals&$3$&$[1\,314,1\,332]$\\
	itn-py&product class~$\times$~intervals&$15$&$[70,510]$\\
	itn-a&animals&$1$&$[210]$\\
	itn-ay&animals in intervals&$3$&$[70,70]$\\
	itn-v&vegetables&$1$&$[796]$\\
	itn-vy&vegetables in intervals&$3$&$[247,262]$\\
	itn-f&food products&$1$&$[1\,137]$\\
	itn-fy&\mbox{food products in intervals}&$3$&$[377,380]$\\
	itn-m&minerals&$1$&$[330]$\\
	itn-my&mineral in intervals&$3$&$[110,110]$\\
	itn-c&chemicals&$1$&$[1\,530]$\\
	itn-cy&chemicals in intervals&$3$&$[510,510]$\\
	\bottomrule
\end{tabular}
\end{table}

\clearpage
